# Supplementary material for: Data Imputation from the Perspective of Graph Dirichlet Energy
Source: arXiv:2304.04474 source file (2024-07-30)
Supplement: Supplementary file 1 [file sec7_appendix.tex]

\section{Datasets} \label{sec:appendA}
We compare our methods with baseline methods using four continuous sensor datasets: METR-LA, NREL, SeData, and PEMS-BAY. METR-LA and PEMS-BAY are released by \cite{li2017diffusion}, focusing on the traffic data recorded in Los Angeles County and Bay Area, respectively. In detail, METR-LA records four months of traffic flow on 207 sensors, and PEMS-BAY records six months of traffic speed on 325 sensors. SeData is another traffic dataset collected by 323 inductive loop detectors deployed on freeways in the Seattle area and published by \cite{cui2018deep, cui2019traffic}. In addition to traffic data, we also utilize NREL for performance assessment, which registers the data from 137 synthetic solar photovoltaic power plants in the United States in 2006. The detailed information is summarized in Table \ref{table:datasets1}

Given that all the datasets are collected in a very long period of time, we use a specific time window to generate the experimental data. To be more specific, in a system with $n$ sensors, the data collected in the length-$h$ time window constitutes the graph with feature matrix $\bm X\in \mathbb{R}^{n\times h}$. Thus, the data collected in non-overlapping time windows could be regarded as different graphs. The graph structures are established by additional side information as follows. For NREL, METR-LA and PEMS, we use a thresholded Gaussian kernel applied to geographic distances following previous works \cite{cini2021filling, wu2021inductive}: We construct the adjacency matrix by $\bm A_{i ,j}=\exp \left(-\left(\frac{\operatorname{dist}\left(v_{i}, v_{j}\right)}{\sigma}\right)^{2}\right),$ where $\operatorname{dist}(v_i,v_j)$ represents the distance between sensor $v_i$ and $v_j$, and $\sigma$ is a normalization factor. For SeData, we construct a binary adjacency matrix defined by $\bm A_{i,j}= \begin{cases}1, & \text { if }v_{i} \text { and } v_{j} \text { are neighbors } \\ 0, & \text { otherwise }\end{cases}$. After a MinMax scaler \cite{rajaraman2011mining}, all the attributes can be scaled to [0,1].

\begin{table}[htb]
\centering
\caption{Summary of continuous sensor datasets.}
\begin{tabular}{ccccc}
\toprule
\textbf{}                & \textbf{METR-LA} & \textbf{NREL} & \textbf{PEMS} & \textbf{SeData} \\ \midrule
Number of Nodes         & 207              & 137           & 325           & 323             \\
Length of Time Window    & 23990            & 36792         & 36481         & 5644            \\
% Number of Graphs              & 975               & 2299           & 1013           & 352              \\ 
\bottomrule
\end{tabular}
\label{table:datasets1}
\end{table}

For real-word graph datasets, Texas and Cornell are two web-page datasets where nodes are the web pages from computer science departments of different universities, and edges are links between pages. ArXiv-Year, Cora and Citeseer are three citation network datasets. YelpChi is a web-page hotel and restaurant review dataset. Table \ref{table:datasets2} shows the detailed statistics.

\begin{table}[htb]
\centering
\caption{Summary of real-word graph datasets.}
\begin{tabular}{ccccccc}
\toprule
\textbf{}                & \textbf{Texas} & \textbf{Cornell} & \textbf{ArXiv-Tear} & \textbf{YelpChi} & \textbf{Cora} & \textbf{Citeseer} \\ \midrule
Number of Nodes         & 183              & 183           & 169,343          & 45,954  & 2,708 & 3,327         \\
Number of Edges         & 309              & 295           & 1,166,243         & 3,846,979  & 5,278 & 4,676         \\
Classes              & 5               &5           & 5          & 2    & 7& 6         \\ 
Node Homophily Ratio  & 0.06 & 0.11           & 0.22  & 0.77 & 0.74 & 0.81             \\
\bottomrule
\end{tabular}
\label{table:datasets2}
\end{table}

SYNTHIE \cite{morris2016faster} is a synthetic dataset consisting of 400 graphs. PROTEINS \cite{borgwardt2005protein} is a dataset of proteins with both continuous features (representing the length in amino acids) and discrete features (labeling the types, namely helix, sheet or loop). FRANKENSTEIN \cite{orsini2015graph} is a small molecules dataset. Each molecule is represented as a graph whose vertices are labeled by the chemical atom symbol and edges are characterized by the bond type. Table \ref{table:datasets3} shows the detailed statistics.

\begin{table}[htb]
\centering
\caption{Summary of multi-graph datasets.}
\begin{tabular}{ccccc}
\toprule
\textbf{}                & \textbf{SYNTHIE} & \textbf{PROTEINS} & \textbf{FRANKENSTEIN}  \\ \midrule
Number of Graphs&400&1113&4337                 \\
Avg. Nodes & 95.00& 39.06&16.90    \\
Avg. Edges  & 172.93  & 72.82  & 17.88    \\

\bottomrule
\end{tabular}
\label{table:datasets3}
\end{table}

% \clearpage
\section{Experimental Setup}
We consider three different imputation settings: 1) Missing Completely At Random (MCAR): For each node, we randomly drop 20\% of the available values of the feature vector;
2) Missing At Random (MAR): First, We randomly select 20\% nodes as "no missing observations". Then we mask out 20\% values of the remaining observations according to a logistic model. 
3) Missing Not At Random (MNAR): We randomly select 20\% nodes as "unobserved observations" and mask out the entire feature vectors of these nodes. The MNAR refers to the situation in which the system wants to introduce several new sensors, or some sensors may break without being replaced. Thus we need to impute the whole feature vectors of these nodes.

We use the Mean Absolute Error (MAE) and Root Mean Squared Error (RMSE) as performance metrics. 
Our models are trained for 800 epochs using an Adam optimizer with a learning rate of 0.001. For the "draft" imputation stage, we use a 1-layer DGCN with 100 hidden units to obtain the rudimentary imputation. We build the residual network using one GDN layer approximated by three-order Maclaurin Series. 
For one pooling-unpooling layer, we set the number of clusters $r$ as {60,80,80,180} for four datasets METR-LA, NREL, PEMS, SeData, respectively. After the reconstruction of GLPN, a 1-layer DGCN is used to get the final results. 

In this work, we compare the performance of our proposed model with the following baselines, which could be further divided into two categories: structure-free methods and structure-based methods.

\noindent \textbf{Structure-free methods}:
\begin{itemize}
[itemsep=2pt,topsep=0pt,parsep=0pt]
\item \textbf{MEAN}: The method imputes the missing value with the mean of all observed features. 
\item \textbf{MF}: The method uses a matrix factorization model to predict the missing values in a matrix.
% \item \textbf{SVD} \cite{troyanskaya2001missing}: The method performs imputation based on matrix completion with iterative low-rank SVD decomposition. 
\item \textbf{Soft} \cite{hastie2015matrix}: The method imputes missing values with iterative soft-thresholded SVD’s.
\item\textbf{MICE }\cite{van2011mice}: The method performs missing value imputation by chained equations.
\item \textbf{OT} \cite{muzellec2020missing}: OT uses the optimal transport distances to quantify the distribution matching and impute missing data.
\item \textbf{GAIN} \cite{yoon2018gain}: GAIN uses a Generative Adversarial Net framework to impute missing data.
\end{itemize}

\noindent \textbf{Structure-based methods}:
\begin{itemize}[itemsep=2pt,topsep=0pt,parsep=0pt]
\item \textbf{KNN}: The method uses the average of K-hop nearest neighbors to serve as imputed values.
\item \textbf{GCN}: The method uses vanilla Graph Convolutional Network \cite{kipf2016semi} to predict missing data.
\item \textbf{GRAPE} \cite{you2020handling}: The method tackles the missing data imputation problem using graph representation based on a deep learning framework.
\item \textbf{GDN} \cite{li2021deconvolutional}: The method uses graph deconvolutional network to recover the missing data via an autoencoder framework.
\item \textbf{VGAE} \cite{kipf2016variational}: The method uses variational auto-encoder (VAE) on graph-structured data.

\end{itemize}

\section{Experiments with Different Draft Strategies}

Given that the draft imputation used to start the model matters a lot, we additionally consider four draft imputation methods, including two structure-free methods (MEAN, Soft) and two structure-based methods (K-hop nearest neighbors, GCN). Note that the model described in the submitted paper utilizes a variant of Graph Convolutional Networks (i.e. DGCN) as the draft component. Similar to Figure 3, we report the normalized results relative to the performance of the MEAN imputation in Table \ref{table:draft_MCAR}, \ref{table:draft_MAR}, \ref{table:draft_MNAR}. Among these strategies, GCN based methods provide the best imputation performance on average. Given that the draft step is not the focus of this work, we only report the best model with DGCN drafter in the paper. It is worth noting that based on all these four draft strategies, GLPN could significantly improve the final imputation performance via an energy-preservation refine step.

\begin{table}[htb]
% {\color{blue}
\caption{Experiments with Different Draft Strategies (MCAR)}
\centering
\begin{tabular}{ccccccccc}
\toprule
\textbf{} &
  \multicolumn{2}{c}{\textbf{METR-LA}} &
  \multicolumn{2}{c}{\textbf{NREL}} &
  \multicolumn{2}{c}{\textbf{PEMS}} &
  \multicolumn{2}{c}{\textbf{SeData}} \\
 &
  RMSE &
  MAE &
  RMSE &
  MAE &
  RMSE &
  MAE &
  RMSE &
  MAE \\ \midrule
Mean &
  1.000 &
  1.000 &
  1.000 &
  1.000 &
  1.000 &
  1.000 &
  1.000 &
  1.000 \\
\textbf{Mean+GLPN} &
  \textbf{0.351} &
  \textbf{0.343} &
  \textbf{0.155} &
  \textbf{0.127} &
  \textbf{0.217} &
  \textbf{0.224} &
  \textbf{0.403} &
  \textbf{0.428} \\ 
Soft &
  0.442 &
  0.389 &
  0.202 &
  0.174 &
  0.554 &
  0.617 &
  0.520 &
  0.574 \\
\textbf{Soft+GLPN} &
  \textbf{0.304} &
  \textbf{0.233} &
  \textbf{0.113} &
  \textbf{0.076} &
  \textbf{0.201} &
  \textbf{0.188} &
  \textbf{0.320} &
  \textbf{0.324} \\ 
KNN &
  0.860 &
  0.805 &
  0.845 &
  0.764 &
  0.906 &
  0.905 &
  0.672 &
  0.645 \\
\textbf{KNN+GLPN} &
  \textbf{0.361} &
  \textbf{0.349} &
  \textbf{0.147} &
  \textbf{0.117} &
  \textbf{0.229} &
  \textbf{0.225} &
  \textbf{0.328} &
  \textbf{0.334} \\ 
GCN &
  0.582 &
  0.595 &
  0.374 &
  0.364 &
  0.594 &
  0.642 &
  0.494 &
  0.537 \\
\textbf{DGCN+GLPN} &
  \textbf{0.284} &
  \textbf{0.270} &
  \textbf{0.097} &
  \textbf{0.051} &
  \textbf{0.180} &
  \textbf{0.182} &
  \textbf{0.319} &
  \textbf{0.327} \\ \bottomrule
\end{tabular}
\label{table:draft_MCAR}
\end{table}

\begin{table}[htb]
% {\color{blue}
\caption{Experiments with Different Draft Strategies (MAR)}
\centering
\begin{tabular}{ccccccccc}
\toprule
\textbf{} &
  \multicolumn{2}{c}{\textbf{METR-LA}} &
  \multicolumn{2}{c}{\textbf{NREL}} &
  \multicolumn{2}{c}{\textbf{PEMS}} &
  \multicolumn{2}{c}{\textbf{SeData}} \\
 &
  \multicolumn{1}{c}{RMSE} &
  \multicolumn{1}{c}{MAE} &
  \multicolumn{1}{c}{RMSE} &
  \multicolumn{1}{c}{MAE} &
  \multicolumn{1}{c}{RMSE} &
  \multicolumn{1}{c}{MAE} &
  \multicolumn{1}{c}{RMSE} &
  \multicolumn{1}{c}{MAE} \\ \midrule
Mean &
  1.000 &
  1.000 &
  1.000 &
  1.000 &
  1.000 &
  1.000 &
  1.000 &
  1.000 \\
\textbf{Mean+GLPN} &
  \textbf{0.368} &
  \textbf{0.298} &
  \textbf{0.139} &
  \textbf{0.095} &
  \textbf{0.172} &
  \textbf{0.182} &
  \textbf{0.447} &
  \textbf{0.443} \\ 
Soft &
  0.667 &
  0.529 &
  0.543 &
  0.360 &
  0.694 &
  0.886 &
  0.680 &
  0.779 \\
\textbf{Soft+GLPN} &
  \textbf{0.291} &
  \textbf{0.204} &
  \textbf{0.152} &
  \textbf{0.085} &
  \textbf{0.225} &
  \textbf{0.188} &
  \textbf{0.317} &
  \textbf{0.318} \\ 
KNN &
  0.890 &
  0.697 &
  0.841 &
  0.667 &
  0.729 &
  0.751 &
  0.567 &
  0.549 \\
\textbf{KNN+GLPN} &
  \textbf{0.371} &
  \textbf{0.305} &
  \textbf{0.131} &
  \textbf{0.086} &
  \textbf{0.176} &
  \textbf{0.184} &
  \textbf{0.313} &
  \textbf{0.319} \\
GCN &
  0.863 &
  0.722 &
  0.743 &
  0.616 &
  0.781 &
  0.847 &
  0.565 &
  0.599 \\
\textbf{DGCN+GLPN} &
  \textbf{0.307} &
  \textbf{0.237} &
  \textbf{0.095} &
  \textbf{0.043} &
  \textbf{0.218} &
  \textbf{0.195} &
  \textbf{0.307} &
  \textbf{0.314} \\ \bottomrule
\end{tabular}
\label{table:draft_MAR}
\end{table}

\begin{table}[htb]
% {\color{blue}
\caption{Experiments with Different Draft Strategies (MNAR)}
\centering
\begin{tabular}{ccccccccc}
\toprule
\textbf{} &
  \multicolumn{2}{c}{\textbf{METR-LA}} &
  \multicolumn{2}{c}{\textbf{NREL}} &
  \multicolumn{2}{c}{\textbf{PEMS}} &
  \multicolumn{2}{c}{\textbf{SeData}} \\
 &
  \multicolumn{1}{c}{RMSE} &
  \multicolumn{1}{c}{MAE} &
  \multicolumn{1}{c}{RMSE} &
  \multicolumn{1}{c}{MAE} &
  \multicolumn{1}{c}{RMSE} &
  \multicolumn{1}{c}{MAE} &
  \multicolumn{1}{c}{RMSE} &
  \multicolumn{1}{c}{MAE} \\ \midrule
Mean &
  1.000 &
  1.000 &
  1.000 &
  1.000 &
  1.000 &
  1.000 &
  1.000 &
  1.000 \\
\textbf{Mean+GLPN} &
  \textbf{0.449} &
  \textbf{0.401} &
  \textbf{0.313} &
  \textbf{0.198} &
  \textbf{0.574} &
  \textbf{0.569} &
  \textbf{0.588} &
  \textbf{0.589} \\
Soft &
  0.519 &
  0.440 &
  0.637 &
  0.552 &
  0.555 &
  0.630 &
  0.878 &
  0.900 \\
\textbf{Soft+GLPN} &
  \textbf{0.300} &
  \textbf{0.584} &
  \textbf{0.325} &
  \textbf{0.223} &
  \textbf{0.641} &
  \textbf{0.695} &
  \textbf{0.651} &
  \textbf{0.670} \\
KNN &
  0.556 &
  0.521 &
  0.401 &
  0.275 &
  0.758 &
  0.758 &
  0.623 &
  0.617 \\
\textbf{KNN+GLPN} &
  \textbf{0.444} &
  \textbf{0.382} &
  \textbf{0.324} &
  \textbf{0.224} &
  \textbf{0.632} &
  \textbf{0.676} &
  \textbf{0.593} &
  \textbf{0.595} \\ 
GCN &
  0.497 &
  0.450 &
  0.699 &
  0.538 &
  0.736 &
  0.728 &
  0.711 &
  0.735 \\
\textbf{DGCN+GLPN} &
  \textbf{0.392} &
  \textbf{0.337} &
  \textbf{0.219} &
  \textbf{0.135} &
  \textbf{0.539} &
  \textbf{0.538} &
  \textbf{0.483} &
  \textbf{0.469} \\ \bottomrule
\end{tabular}
\label{table:draft_MNAR}
\end{table}

%\color{blue}{}

\section{Dirichlet Energy Changes under Different Missing Mechanisms}

\begin{figure*}[htb]
  \centering
  \includegraphics[width=\textwidth]{AAAI_Experiments/energy_threesetting2.pdf}
  
  \caption{The Dirichlet energy of different imputation strategies on three experimental datasets (METR-LA, PEMS, NREL) with different missing ratios under three experimental missing mechanisms (MCAR, MAR, MNAR). Relative Dirichlet energy is normalized by that of the ground truth features.}
  \vspace{-2mm}
    \label{fig:app}
\end{figure*}

Empirically, as shown in Figure \ref{fig:app}, imputation strategies during the "draft" step (Mean, KNN) will lead to the Dirichlet energy reduction under all the three experimental data missing mechanisms (MCAR, MAR, MNAR).

\section{Proof for Equation (2)} \label{proof: Equation 2}
Equation (2) connects the graph Dirichlet energy with the quality of imputation.
\begin{equation*}
\parallel\hat{\bm X} - \bm X\parallel \geq \frac{|E_D(\hat{\bm X}) - E_D(\bm X)|}{2B\lambda_{\max}},
\end{equation*}
where $B = \max(\parallel\hat{\bm X}\parallel, \parallel\bm X\parallel)$, and $\lambda_{\max}$ is the largest eigenvalue of $\tilde{\Delta}$ which is smaller than 2. 
\label{proof:eq2}
\begin{proof}
Let $E_D(\bm X)=tr\left(\bm X^T \tilde{\Delta} \bm X\right)$ be the Dirichlet energy, $\bm X_a$ and $\bm X_b$ be two bounded feature matrices, and $B = \max\left(\parallel \bm X_a\parallel, \parallel\bm X_b\parallel\right)$ be the $\ell_2$ boundary. Consider that $E_D(\bm X)$ is a local Lipschitz function when $\bm X$ is bounded, we have:
\begin{equation*}
    \begin{aligned}
    \frac{|E_D(\bm X_a) - E_D(\bm X_b)|}{\parallel \bm X_a - \bm X_b \parallel} \leq & \sup_{\parallel \bm X\parallel \leq B} \parallel \frac{\partial E_D(\bm X)}{\partial \bm X} \parallel\\
    = & \sup_{\parallel \bm X\parallel \leq B} \parallel 2\tilde{\Delta} \bm X \parallel\\
    \leq & ~ 2 \lambda_{max} B.
    \end{aligned}
\end{equation*}
\end{proof}

\section{Proof of Proposition 2} 
\label{proof:proposition 2}
% \begin{proposition}{2}
% \label{proposition2}
\textbf{Proposition 2.} 
\textit{Suppose each element in} $\bm X$ \textit{is identically independent drawn from a certain distribution whose first and second moment constraints satisfy} $\mathbb E(\bm X_{i,j}) = 0$ \textit{and} $\text{Var}(\bm X_{i,j}) = 1$,\textit{ and the imputation} $\hat{\bm X}$ \textit{satisfy} $\hat{\bm X}_{i,j}=\sum_{k\in S_k}\alpha_{k}\bm X^{\star}_{i,k}$,\textit{ where} $\sum_{k\in S_k} \alpha_{k}=1$, $\alpha_k \geq 0$, and $S_k = \{1\leq k \leq N|M_{ik}=1\}$, \textit{we have} $\mathbb E[E_D(\hat{\bm X})] \leq \mathbb E[E_D(\bm X)]$.
% \end{proposition}

\begin{proof}
We first consider the case that $\bm X$ only has one feature column, i.e., $\bm X \in \mathbb R^{N\times 1}$. According to Equation (1), if $\bm X_i$ and $\bm X_j$ are connected, the related term in the graph Dirichlet energy is
\begin{equation*}
    e_D\left(\bm X_i,\bm X_j\right)=\left(\dfrac{\bm X_{i}}{\sqrt{1+\bm D_{i,i}}}-\dfrac{\bm X_{j}}{\sqrt{1+\bm D_{j,j}}}\right)^2.
\end{equation*}

\noindent Using the first and second moment constraints of $\bm X_i$ and $\bm X_j$, the expectation of $e_D(\bm X_i,\bm X_j)$ can be calculated by
\begin{equation*}
    \mathbb E\left(e_D(\bm X_i,\bm X_j)\right)=\text{Var}\left(\dfrac{\bm X_{i}}{\sqrt{1+\bm D_{i,i}}}\right)+\text{Var}\left(\dfrac{\bm X_{j}}{\sqrt{1+\bm D_{j,j}}}\right) =
    \frac{1}{1+\bm D_{i,i}}+\frac{1}{1+\bm D_{j,j}}.
\end{equation*}

\noindent If $\bm X_i$ is missing and imputed by $\hat{\bm X}_{i}=\sum_{k\in S_k}\alpha_{k}\bm X_{k}$ while $\hat{\bm X_j}=\bm X_j$ is unchanged, we have
\begin{equation*}
\begin{aligned}
\mathbb E\left(e_D(\hat{\bm X}_{i},\hat{\bm X_j})\right)\leq& \text{Var}\left(\dfrac{\sum_{k\in S_k}\alpha_{k}\bm X_{k}}{\sqrt{1+\bm D_{i,i}}}\right)+\text{Var}\left(\dfrac{\bm X_{j}}{\sqrt{1+\bm D_{j,j}}}\right)\\
\leq& \frac{\sum_{k\in S_k}\alpha_{k}^2}{1+\bm D_{i,i}}+\frac{1}{1+\bm D_{j,j}} \\
\leq& \frac{1}{1+\bm D_{i,i}}+\frac{1}{1+\bm D_{j,j}}.
    \end{aligned}
\end{equation*}

\noindent On the other side, if both $\bm X_i$ and $\bm X_j$ are missing and imputed by $\hat{\bm X}_{i}=\sum_{k\in S_k}\alpha_{k}\bm X_{k}$ and $\hat{\bm X}_{j}=\sum_{k\in S_k}\beta_{k}\bm X_{k}$ respectively, we have

\begin{equation*}
\begin{aligned}
\mathbb E\left(e_D(\hat{\bm X}_{i},\hat{\bm X_j})\right)\leq& \text{Var}\left(\dfrac{\sum_{k\in S_k}\alpha_{k}\bm X_{k}}{\sqrt{1+\bm D_{i,i}}}\right)+\text{Var}\left(\dfrac{\sum_{k\in S_k}\beta_{k}\bm X_{k}}{\sqrt{1+\bm D_{j,j}}}\right)\\
\leq& \frac{\sum_{k\in S_k}\alpha_{k}^2}{1+\bm D_{i,i}}+\frac{\sum_{k\in S_k}\beta_{k}^2}{1+\bm D_{j,j}} \\
\leq& \frac{1}{1+\bm D_{i,i}}+\frac{1}{1+\bm D_{j,j}}.
    \end{aligned}
\end{equation*}

\noindent In summary, we have
\begin{equation}
    \mathbb E[E_D(\hat{\bm X})]=\sum_{\{(i,j)|\bm A_{ij}=1\}}E(e_D(\hat{\bm X}_{i},\hat{\bm X_j})) \leq \sum_{\{(i,j)|\bm A_{ij}=1\}}E(e_D(\bm X_{i},\bm X_j))\leq \mathbb E[E_D(\bm X)].
\end{equation}

\noindent Similarly, if $\bm X$ has more than one feature column, i.e., $\bm X \in \mathbb R^{N\times d}$, we have $\mathbb E[E_D(\hat{\bm X}_{i,:})]\leq \mathbb E[E_D(\bm X_{i,:})]$ for $0\leq i < d$, and thus $\mathbb E[E_D(\hat{\bm X})]\leq \mathbb E[E_D(\bm X)]$.

\end{proof}

\section{Proof for Proposition 3}  \label{Proof:Proposition 3}

\textbf{Proposition 3}. 
\textit{If we use the first-order Maclaurin Series approximation of GDN as the residual layer, the Dirichlet energy of one layer {simplified} GLPN {without the weight matrix} is bounded as follows: }
\begin{equation} 
(1 + C_{min})^2 E_D(\bm X_d) \leq E_D (\hat{\bm X}),
\end{equation}
\noindent \textit{where} $C_{min}$ \textit{is the minimum eigenvalue of matrix} $\tilde{\Delta}+\alpha \bm S\bm S^T$.

\begin{proof}
As illustrated in Section 5.2, for the proposed GLPN with one-level pooling-unpooling, the output of our model could be formulated by: 
\begin{equation*}
    \hat{\bm X}=\bm P_l \bm X_d+ \alpha \bm S\bm S^T\bm X_d.
    % \label{eq.pyramid_layer1}
\end{equation*}
We define $\bm Q \triangleq \bm P_l+ \alpha \bm S\bm S^T$, and then simplify the above expression as 
\begin{equation*}
    \hat{\bm X}=\bm Q \bm X_d  .
\end{equation*}
We represent the decomposition of matrix $\bm Q$ as: $\bm Q = \bm U \bm \Lambda \bm U^{T}$, where the columns of $\bm U$ constitute
an orthonormal basis of eigenvectors of $\bm Q$, and the diagonal matrix $\bm \Lambda$ is comprised of the corresponding eigenvalues of $\bm Q$. 

\noindent For $E_D(\hat{\bm X})$, we have:
\begin{equation*}
\begin{split}
E_D(\hat{\bm X})& =\operatorname{tr} \left(( \bm U \bm \Lambda\bm U^T \bm X_d)^T \tilde{\Delta} (\bm U \bm \Lambda\bm U^T \bm X_d) \right) \\
& = \operatorname{tr}\left (\bm X^T_d \bm U \bm \Lambda\bm U^T \tilde{\Delta} \bm U \bm \Lambda\bm U^T \bm X_d\right)\\
& = \operatorname{tr}\left(\bm U^T \bm X_d \bm X^T_d \bm U \bm \Lambda\bm U^T \tilde{\Delta} \bm U \bm \Lambda\right) \\
& \geq \delta \operatorname{tr}\left(\bm U^T \bm X_d \bm X^T_d \bm U \bm \Lambda\bm U^T \tilde{\Delta} \bm U\right) \\
& = \delta \operatorname{tr}\left(\bm \Lambda\bm U^T \tilde{\Delta} \bm U \bm U^T \bm X_d \bm X^T_d \bm U\right) \\
& \geq {\delta}^2 \operatorname{tr}\left(\bm X_d^T \tilde{\Delta} \bm X_d\right) \\
& = {\delta}^2 E_D(\bm X_d),
\end{split}
\end{equation*}
where $\delta$ is the minimum eigenvalue of matrix $\bm Q$. 
Recalling $\bm Q\triangleq \bm P_l+ \alpha \bm S\bm S^T$ and $\bm P_l\triangleq\bm I+\tilde{\Delta}$, then we have $\delta = 1+C_{min}$, where $C_{min}$ is the minimum eigenvalue of matrix $\tilde{\Delta} + \alpha \bm S\bm S^T$.

\noindent In summary, we have
\begin{equation*}
 (1 + C_{min})^2 E_D(\bm X_d) \leq E_D (\hat{\bm X})   ,
\end{equation*}
where $C_{min}$ is the minimum eigenvalue of matrix $\tilde{\Delta}+\alpha \bm S\bm S^T$.

\end{proof}

\section{Proposition 3 with Higher-order Maclaurin Series Approximation }\label{Proof:Proposition 3 Higher}
Although we adopt the first-order Maclaurin series approximation of GDN in analysis, we can obtain similar results in the higher-order approximation. For example, using the second-order Maclaurin Series approximation, Equation (10) would be $$\hat{\bm X}=\tilde{\bm P}_l  \bm X_d+ \alpha  \bm S \bm S^T \bm X_d,$$ where $ \tilde{\bm P}_l= \bm I+\tilde{\Delta}+\frac{1}{2}{\tilde{\Delta}}^2$. Then, we have a similar conclusion for Proposition 3:
$$(1 + \tilde{C}_{min})^2 E_D(\bm X_d) \leq E_D (\hat{\bm X}), $$ 
where $\tilde{C}_{min}$ is the minimum eigenvalue of matrix $\tilde{\Delta}+\frac{1}{2}{\tilde{\Delta}}^2+\alpha \bm S \bm S^T$.
